# Supplementary material for: Diffusion backbone of temporal higher-order networks
Source: arXiv:2412.12856 source file (2024-12-17)
Supplement: Supplementary file 1 [file Appendix.tex]

% \section*{Appendix}
% \newpage
\appendices
\onecolumn
\begin{figure}[h]
    \centering
    \includegraphics[scale=0.8]{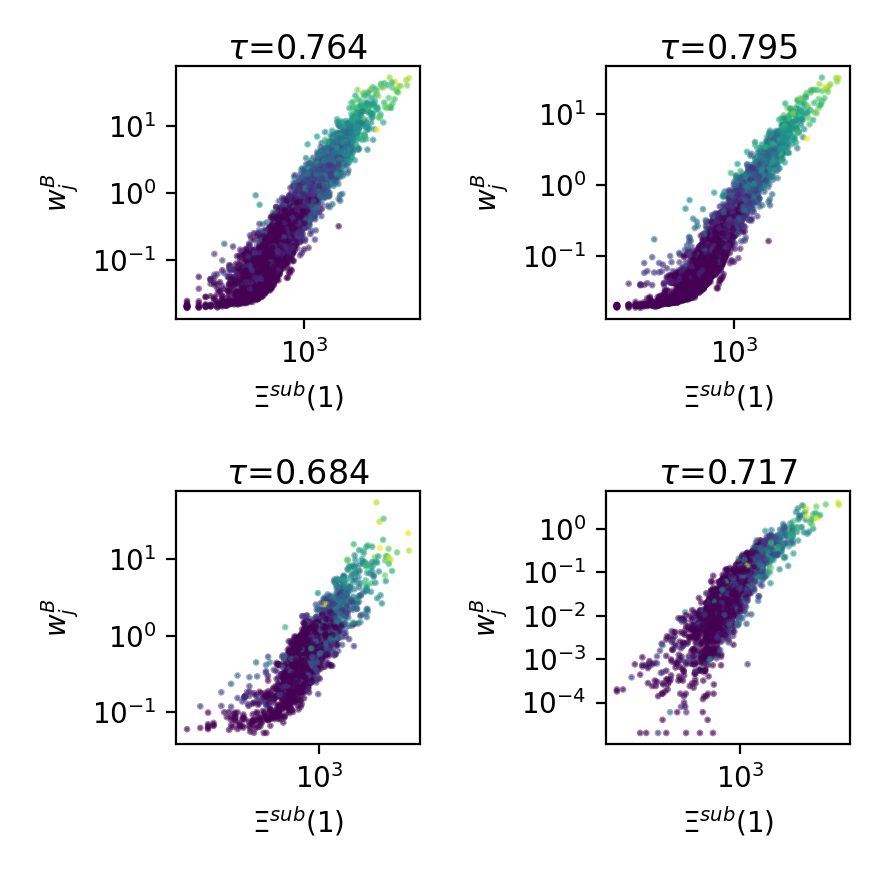}
    \caption{$\beta=10^{-2}$. $w_j^B$ versus $\Xi_j^{adj}(1)$. Top (botttom) panels correspond to order 2 (order 3). Left and right panels correspond to $\Theta=1$ and $\Theta=d-1$.}
    \label{sfig:wj}
\end{figure}
\begin{figure}[h]
    \centering
    \includegraphics[scale=0.9]{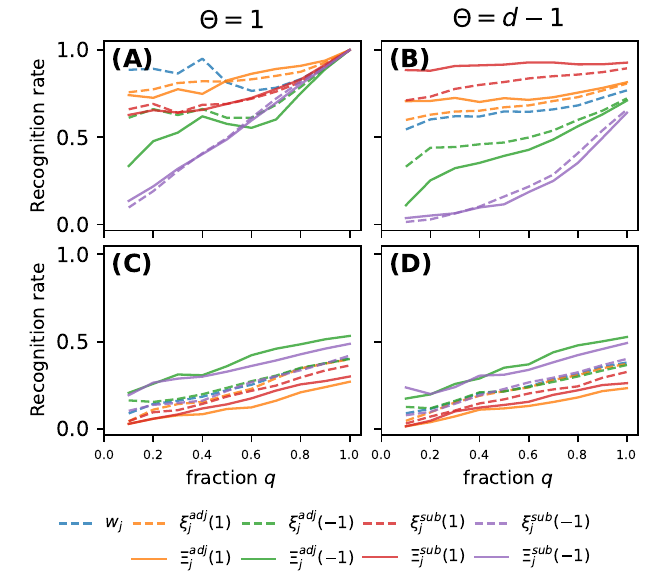}
    \caption{Recognition rate of a local metric in recognizing top-$q$ triadic hyperlinks in the backbone $B$ as a function of fraction $q$, when $\beta=10^{-3}$ (A-B) and $\beta=1.0$ (C-D), on SFHH dataset. Two columns corresponds to $\Theta=1$ and $\Theta=d-1$, respectively.  The dashed (solid) lines correspond to time-independent (time-dependent) metrics.}
    \label{fig:SFHH_recog}
\end{figure}
\section{Analytical analysis of backbone weights for small $\beta$}
The diffusion backbone is the union of all $|\mathcal{N}|$ diffusion trajectories that start from one seed node, i.e., $B=\cup_{i}\mathcal{T}_i$. We illustrate that when the infection probability $\beta$ approaches zero, each diffusion trajectory $\mathcal{T}_i$ can be approximated by the local interaction of the seed node $i$ in the aggregated network $H$, which allows us to derive approximation of weights $w_j^B$ of a hyperlink as $\beta\rightarrow 0$.
 In the following, we will show that the weight $w_j^B$ in the backbone $B$ can be approximated by the weight $w_j$ in the aggregated higher-order network $H$ in the limit of $\beta\rightarrow 0$, in the two cases of threshold $\Theta$. Taking order-3 hyperlinks as an example, i.e., $d_j=3$, we will derive the linear and quadratic approximations of $w_J^B$ in terms of $\beta$, using the local information of the temporal higher-order network.
% We define the $0$-hop neighborhood of a hyperedge $\mathcal{E}_j$ as a subgraph that consists of all higher-order edes among a subset of nodes in $\mathcal{E}_j$, in the aggregated higher-order network.
% \subsection{First order approximation of weight $w_j^B$}

% \begin{figure}[ht!]
%     \centering
%     \subfloat[$0$-hop neighborhood]{
%          \centering
%         \input{figs/triangle1.tikz}
%          % \subcaption{$0$-hop neighborhood of a order-3 hyperlink.}
%          \label{fig:0hop}
%     }
%     % \hfill
%     \subfloat[$1$-hop neighborhood]{
%          % \centering
%         \input{figs/triangle2.tikz}
%          % \subcaption{$1$-hop neighborhood of a order-3 hyperlink.}
%     % \label{fig:order3edge2}
%          \label{fig:1hop}
%     }
%     % \input{figs/triangle1.tikz}
%     \caption{Considering $0$-hop neighborhood of a hyperedge $j$ with three nodes.}
%     \label{fig:order3edge1}
% \end{figure}

Let us rewrite the definition of $w_j^B$:
\begin{align*}
    w_j^B = & \frac{1}{|\mathcal{N}|}\sum_{i\in \mathcal{N}} w_j^{\mathcal{T}_i}
\end{align*}
As $\beta\rightarrow 0$, we approximate the backbone as the union of the diffusion trajectories that contributes to the weight $w_j^B$ to the order of $\beta$ (linear) and $\beta^2$ (quadratic), and other diffusion trajectories are ignored since their contribution is negligible as $\beta\rightarrow 0$. These relevant diffusion trajectories either start from a node in $j$ as shown in Figure \ref{fig:0hop}, or from $j$'s 1-hop neighbor as shown in Figure \ref{fig:1hop}
\subsection{\textbf{Threshold $\Theta=1$}}
By using the conditional expectation, we derive the approximation of the weight $w_j^{\mathcal{T}_i}$ in trajectory $\mathcal{T}_i$ when the seed node $i$ belongs to the hyperlink $h_j$:
\begin{align*}
    w_j^{\mathcal{T}_i}\approx & \left[2\cdot Pr(j\text{ is activated twice}|i\text{ is the seed}) + Pr(j\text{ is activated once}|i\text{ is the seed})  \right] \\
    \approx &\left (1-w_1\beta\right )\left (1-w_2\beta\right )(w_j\beta)^2\cdot2  \\
    &+\left (1-w_1\beta\right )\left (1-w_2\beta\right )\cdot 2w_j\beta (1-w_j\beta)+(1-w_1\beta)w_2\beta w_j\beta+w_1\beta(1-w_2\beta)w_j\beta \\
    % &+(1-w_1\beta)w_2\beta\cdot w_j\beta+(1-w_2\beta)w_1\beta\cdot w_j\beta \\
    % &+... \\\
    =&2w_j\beta+\left (2w_j^2-2w_jw_1-2w_jw_2-2w_j^2+w_2w_j+w_1w_j\right )\beta^2 + o(\beta^2) \\
    =&2w_j\beta-w_j\left (w_1+w_2\right )\beta^2 + o(\beta^2) 
   % \langle w_j^B\rangle \approx &\left (6-2w_{|\subset j}\beta\right )w_j\beta \approx 6 e^{-\frac{1}{3}\beta w_{|\subset j}}\cdot w_j\beta\approx \frac{6}{1+\frac13 \beta w_{|\subset j}} w_j \beta
\end{align*}
and when the seed node $i$ is $h_j$'s 1-hop neighbor:
\begin{align*}
    w_j^{\mathcal{T}_i}\approx &w_0\beta\cdot2w_j \beta+o(\beta^2)=2w_0w_j\beta^2+o(\beta^2)\\
   % \langle w_j^B\rangle \approx &\left (6-2w_{|\subset j}\beta\right )w_j\beta \approx 6 e^{-\frac{1}{3}\beta w_{|\subset j}}\cdot w_j\beta\approx \frac{6}{1+\frac13 \beta w_{|\subset j}} w_j \beta
\end{align*}
% By applying the conditional expectation, we can calculate the contribution of diffusion trajectories that starts from $j$'s 1-hop neighbor:
% \begin{align*}
%     % w_j^B\approx & w_0\beta\cdot 2w_j\beta (1-w_j\beta) + w_0'\beta\cdot 2w_j\beta (1-w_j\beta) + w_0''\beta\cdot 2w_j\beta (1-w_j\beta) \\
%     w_j^B\approx & w_0\beta\cdot 2w_j\beta (1-w_j\beta) + o(\beta^2)\\
%     =& w_0\cdot 2w_j\cdot \beta^2 + o(\beta^2)\\
% \end{align*}
By adding up the contribution from the above two terms, we have:
\begin{align*}
    w_j^B\approx &\frac{1}{|\mathcal{N}|}\left(2w_j\beta-w_j\left (w_1+w_2\right )\beta^2 
     +2w_j\beta-w_j\left (w_2+w_3\right )\beta^2 
    +2w_j\beta-w_j\left (w_3+w_1\right )\beta^2 + 2w_0w_j\beta^2 + o(\beta^2) \right)
    \\
    = & \frac{1}{|\mathcal{N}|}\left(6w_j\beta+2w_j(w_0-w_1-w_2-w_3)\beta^2+o(\beta^2) \right )\\
    % & w_0\beta\cdot 2w_j\beta (1-w_j\beta) + w_0'\beta\cdot 2w_j\beta (1-w_j\beta) + w_0''\beta\cdot 2w_j\beta (1-w_j\beta) \\
    % w_j^B\approx & w_0\beta\cdot 2w_j\beta (1-w_j\beta) + o(\beta^2)\\
    = & \frac{1}{|\mathcal{N}|}\left [6\beta + 2(w_0-w_1-w_2-w_3)\cdot  \beta^2 + o(\beta^2)\right ]\cdot w_j\\
\end{align*}
\subsection{\textbf{Threshold $\Theta=d-1$}}
% \subsection{Contribution of the $0$-hop neighborhood of a hyperedge}
% When the infection probability $\beta$ is close to $0$, the contribution to the link weight in backbone $w_j^B$ mainly comes from the $0$-hop neighborhood.
Similarly, we first consider the cases when the seed node is inside hyperlink $j$.
 % we denote the link weights of the three pairwise sublinks in the aggregated network as $w_{v}$, where $v=1,2,3$. Since each hyperlink can infect at most one susceptible node ($\Theta=h-1$), weight $w_j^B$ can be approximated as the sum of probabilities that hyperlink $j$ is activated under the condition the seed node is one of the three nodes:
\begin{align*}
    w_j^{\mathcal{T}_i} \approx & Pr(j\text{ is activated once}|i\text{ is the seed} ) \\
    \approx&\left (w_1\beta-\frac{w_1(w_1-1)}{2}\beta^2 \right )\left (1-w_2\beta \right )\left (1-w_3\beta \right )w_j\beta + \left (w_2\beta-\frac{w_2(w_2-1)}{2}\beta^2 \right )\left (1-w_1\beta \right )\left (1-w_3\beta \right )w_j\beta + o(\beta^3)\\
    =&w_1w_j\beta^2-\frac{w_1w_j(w_1+2w_2+2w_3-1)}{2}\beta^3 + w_2w_j\beta^2-\frac{w_2w_j(w_2+2w_1+2w_3-1)}{2}\beta^3 +o(\beta^3)\\
    =&(w_1+w_2)w_j\beta^2-\left (2(w_1+w_2+w_3)^2-(w_1^2+w_2^2+w_3^2)-(w_1+w_2+w_3)\right )w_j\beta^3+o(\beta^3) \\
    w_j^B \approx & \sum_{s\in h_j}Pr(j\text{ is activated once}|s\text{ is the seed} ) \\
    \approx&\left (w_1\beta-\frac{w_1(w_1-1)}{2}\beta^2 \right )\left (1-w_2\beta \right )\left (1-w_3\beta \right )w_j\beta + \left (w_2\beta-\frac{w_2(w_2-1)}{2}\beta^2 \right )\left (1-w_1\beta \right )\left (1-w_3\beta \right )w_j\beta \\
    &+ \left (w_2\beta-\frac{w_2(w_2-1)}{2}\beta^2 \right )\left (1-w_3\beta \right )(1-w_1\beta)w_j\beta + \left (w_3\beta-\frac{w_3(w_3-1)}{2}\beta^2 \right )\left (1-w_2\beta \right )(1-w_1\beta)w_j\beta \\
    &+ \left (w_3\beta-\frac{w_3(w_3-1)}{2}\beta^2 \right )\left (1-w_1\beta \right )(1-w_2\beta)w_j\beta + \left (w_1\beta-\frac{w_1(w_1-1)}{2}\beta^2 \right )\left (1-w_3\beta \right )(1-w_2\beta)w_j\beta \\
    =&w_1w_j\beta^2-\frac{w_1w_j(w_1+2w_2+2w_3-1)}{2}\beta^3 + w_2w_j\beta^2-\frac{w_2w_j(w_2+2w_1+2w_3-1)}{2}\beta^3 \\
    &+w_2w_j\beta^2-\frac{w_2w_j(w_2+2w_3+2w_1-1)}{2}\beta^3 +w_3w_j\beta^2-\frac{w_3w_j(w_3+2w_2+2w_1-1)}{2}\beta^3 \\
    &+w_3w_j\beta^2-\frac{w_3w_j(w_3+2w_1+2w_2-1)}{2}\beta^3 +w_1w_j\beta^2-\frac{w_1w_j(w_1+2w_3+2w_2-1)}{2}\beta^3 + o(\beta^3) \\
    =&2(w_1+w_2+w_3)w_j\beta^2-\left (2(w_1+w_2+w_3)^2-(w_1^2+w_2^2+w_3^2)-(w_1+w_2+w_3)\right )w_j\beta^3+o(\beta^3) \\
    =&2(w_1+w_2+w_3)w_j\beta^2+o(\beta^2)
    % =&2w_{|\subset j}w_j\beta^2-\left (w_{|\subset j}^2-w_{|\subset j}\right )w_j\beta^3+o(\beta^3) \\
    \\
    % \langle w_j^B\rangle \approx 2&\left (1-w_{|\subset j}\beta\right )w_{|\subset j}w_j\beta^2 \approx 2 e^{-\beta w_{|\subset j}}\cdot w_{|\subset j} w_j\beta^2\approx 2\frac{1}{1+\beta w_{|\subset j}}w_{|\subset j}w_j\beta^2
    % w_j^B \approx &\left (2-w_{|\subset j}\beta+\beta\right )w_{|\subset j}w_j\beta^2 \\
\end{align*}
% where $w_{|\subset j}=w_1+w_2+w_3$. When the seed node is outside the hyperlink $j$, the probability of hyperlink $j$ to be activated is to the order of $\beta^3$, which can thus be ignored for small $\beta$, the weight $w_j^B$ is order .
The contribution of the case where the seed node is $j$'s 1-hop neighbor:
\begin{align*}
    w_j^B\approx &w_0\beta\cdot \sum_{s\in h_j}Pr(j\text{ is activated once}|s\text{ is the seed} ) \\
    \approx & 2w_0 (w_1+w_2+w_3)w_j\beta^3 + o(\beta^3) 
    % w_j^B \approx  \\
    % w_j^B \approx &\left (2-w_{|\subset j}\beta+\beta\right )w_{|\subset j}w_j\beta^2 \\
\end{align*}
By adding up the above two terms:
\begin{align*}
    w_j^B\approx & 2(w_1+w_2+w_3)w_j\beta^2 + o(\beta^2) \\
    = & \left [2(w_1+w_2+w_3)\beta^2 + o(\beta^2) \right ]\cdot w_j
    % w_j^B \approx  \\
    % w_j^B \approx &\left (2-w_{|\subset j}\beta+\beta\right )w_{|\subset j}w_j\beta^2 \\
\end{align*}
% \textbf{Threshold $\Theta=1$.} 
% \subsection{Contribution of the $1$-hop neighorhood of a hyperedge}

% \begin{figure}[ht!]
%     \centering
%     \input{figs/triangle2.tikz}
%     \caption{Considering $1$-hop neighborhood of a hyperedge with three nodes.}
%     \label{fig:order3edge2}
% \end{figure}
